# Supplementary material for: FOCAL: Contrastive Learning for Multimodal Time-Series Sensing Signals in Factorized Orthogonal Latent Space
Source: arXiv:2310.20071 source file (2023-10-30)
Supplement: Supplementary file 1 [file rebuttal_responses.tex]

\newcommand{\tommy}[1]{{\color{orange}TOMMY: #1}}
\section{Rebuttal Responses}

\subsection{General Responses}
We would like to sincerely thank all the reviewers for their valuable feedback and constructive suggestions for this submission. As a summary of our responses, we have finished the following tasks during the rebuttal period:

\begin{enumerate}
    \item We added a sensitivity test of loss hyperparameters on ACIDS and PAMAP2 datasets, including three loss weight terms ($\lambda_p$, $\lambda_o$, $\lambda_t$) and the temporal constraint margin. We present the accuracy of \model with different hyperparameters in Figure \ref{fig:sensitivity_test}, and the results show that FOCAL is generally resilient against these hyperparameters. Therefore, the hyperparameter values are mostly shared across different datasets and backbone encoders, with manual tuning only on temporal constraint weight $\lambda_t$. In addition, we set the private loss weight $\lambda_p$ as 1, the orthogonal loss weight $\lambda_o$ as 3, and the temporal loss margin as $1$ by default. 
    \item As suggested by Reviewer zwVA, we applied the proposed temporal constraint to multiple baselines (i.e., SimCLR, MoCo, CMC, Cocoa, and GMC), and achieved noticeable performance improvement compared to their vanilla versions. The full results on ACIDS and PAMAP2 datasets are summarized in Table \ref{tab:temporal_constraints_baselines_acids} and Table \ref{tab:temporal_constraints_baselines_pamap2}. The inspiring results demonstrated the effectiveness of the proposed temporal constraint in general contrastive learning frameworks for time-series data.
    \item We provided the visualization comparison between FOCAL and several multi-modal contrastive baselines in Figure \ref{fig:tsne_deepsense} and Figure \ref{fig:tsne_sw_t}, which showed that FOCAL achieved better separation among different downstream classes after the pretraining.
    \item Due to the space limit, we have put the discussion of technical limitations and potential extensions in Appendix \ref{appendix:limitations}, and we will accordingly expand this list by integrating the comments of all reviewers.
    \item We promise to fix all presentation and terminology issues pointed out by Reviewer Q2hY.
\end{enumerate}

Below, we also respond to each reviewer's comments individually.

\subsection{Reviewer zwVA}

\textcolor{blue}{Q: It would be very strong to show that the proposed loss serves as a plugin that enhances other contrastive learning methods.}

Response: Thanks for the suggestion. We have applied the proposed temporal constraint to multiple contrastive learning baselines (i.e., SimCLR, MoCo, CMC, Cocoa, and GMC). Table \ref{tab:temporal_constraints_baselines_acids} and \ref{tab:temporal_constraints_baselines_pamap2} summarize the results on ACIDS and PAMAP2, and we have observed noticeable performance improvement in most cases (up to 18.99\% on ACIDS and up to 8.39\% on PAMAP2). It validates that the temporal constraint can be used as a plugin to enhance existing contrastive learning frameworks for time-series data.

\textcolor{blue}{Q: The paper discussed little on the technical limitation and future directions. It would be great the discuss more on failure cases.}

Response: We would like to note that the limitations and potential extensions of this paper are discussed in Appendix \ref{appendix:limitations}. We will also expand this list by integrating the comments made by all reviewers in the next version.

\subsection{Reviewer WTA9}

\textcolor{blue}{Q: Is there any hyperparameter search performed for $\lambda_p$, $\lambda_o$, and $\lambda_t$ which control the weights of each loss component? Additionally, was there any hyperparameter search carried out for other methods?}

Response: We did not perform an extensive hyperparameter search for the loss weights in FOCAL, which we agree might slightly improve our performance. Instead, we manually tune the hyperparameters on one dataset and use the same hyperparameters across the remaining datasets, with minor changes (i.e., on $\lambda_t$). The same tuning strategy is also carried out for all baseline methods. As mentioned in our general response, we have added the sensitivity test results in Figure \ref{fig:sensitivity_test} to demonstrate the resiliency of FOCAL against these hyperparameter values.

\textcolor{blue}{Q: Why does the FOCAL-wDistInd perform worse than the noOrth model? Does the replacement of orthogonality with distributional independence contribute to this difference?}

Response: As we observed in the experiment, the distributional independence constraint leads to significant performance degradation in most cases, even worse than the FOCAL-noOrth, especially when SwinTransformer is used as the backbone encoder. Our interpretation is two-fold: First, the dynamic nature of the attention mechanism within SwinTransformer makes the distribution of encoded latent features more complicated; Second, the iterative training between the distribution discriminator and the contrastive objectives does not work coherently as with the autoencoder training. We leave the effective integration of distributional disentanglement and contrastive learning framework as a future exploration direction.

\subsection{Reviewer oGNZ}

\textcolor{blue}{Q: I wonder if some of the training objectives may compete during training, and how do the authors set the three hyper-parameters $\lambda_p$, $\lambda_o$, and $\lambda_t$? Does it require some manual hyperparameter tuning? Jointly optimizing the four objectives does not look like an easy task.}

Response: Our conclusion is that competition between learning objectives does not happen in FOCAL, for the following reasons. First, without the private space task, the performance of FOCAL-noPrivate is much lower than FOCAL-noOrth (note noPrivate also implicitly means no orthogonality constraint), thus the private contrastive loss contributes positively to FOCAL. Second, for the orthogonality constraint and temporal constraint, FOCAL works better than FOCAL-noOrth and FOCAL-noTemp variants respectively, thus our orthogonal constraint and temporal constraint both contribute positively. Instead, we observed that FOCAL-wDistInd works worse than FOCAL-noOrth, while FOCAL-wTempCon works worse than FOCAL-noTemp, which means the competition happens between these alternative constraints and the original contrastive objectives. As for the hyper-parameters, they are mostly shared across different datasets and backbone encoders. We set $\lambda_p$ as 1 and $\lambda_o$ as 3 by default and only tune $\lambda_t$ manually when needed. As mentioned in our general response, we have added the sensitivity test results to demonstrate the resiliency of FOCAL against these hyperparameter values.

\subsection{Reviewer Q2hY}

\textcolor{blue}{Q: The biggest concern is the effectiveness of multimodal feature factorization. From line 161, this work uses the simple soft orthogonal constraint to decouple or factorize each modality feature. However, the single orthogonal constraint is too simple and may not decouple multimodal features well. In particular, information is easily leaked between modalities, and many prior works have tried to solve this problem such as [1-3]. In addition, there is no visualization result for both subspaces in the experimental part, so it is difficult to determine whether the factorization is effective.}

Response: We agree with the reviewer that FOCAL shares with reference [1-3] in exploiting both shared information and private information in multi-modal collaboration. However, there are several factors that make FOCAL substantially different from the listed references. 
First, regarding the learning paradigm, [1, 2, 3] all work with supervised tasks (classification or reconstruction) where the disentanglement objectives are used as augmentations to original task objectives. However, FOCAL works with self-supervised contrastive learning, where the factorization space should be designed without knowledge of downstream tasks and the auxiliary objectives should cooperate with the contrastive learning objectives, which are challenges that have not been considered in listed references.
Second, regarding the application scenario, we have positioned the paper as a self-supervised learning framework for multi-model time-series sensing signals where contributions are made from both the multi-modal perspective and time-series perspective. While we think part of the design could be potentially applicable to more diverse application scenarios, the evaluation of language-vision-acoustics task is beyond the scope of this paper and we leave it as our future explorations. 

We select the simple orthogonal constraint according to the intuition that it aligns well with the contrastive learning paradigm and the fact that it benefits the downstream task performance. 
On the one hand, contrastive learning works in a manner that the angular similarity between embeddings represents semantical proximity, while the geometrical orthogonal constraint is aligned with semantical independence in contrastive learning and penalizes the overlaps between the private space and shared space.
On the other hand, adding orthogonal constraints benefits the downstream tasks after the contrastive pretraining phase. As we presented in the ablation study, although the alternative distributional independence might create better-disentangled representations, it leads to significant degradation after being integrated with the contrastive objectives. 

As for the information leakage concern (i.e., exactly the same information is exploited in both spaces), we believe the proposed orthogonal constraint is a valid solution that prevents leakage while being suitable for contrastive learning, as demonstrated by the end results in our ablation study. The performance improvement of FOCAL-noOrth to FOCAL-noPrivate means the private space task encourages the encoder to exploit more comprehensive semantics, while the improvement of FOCAL to FOCAL-noOrth further validates that the orthogonal constraint encourages the private space to exploit non-overlapped information as the shared space and enriches the learned semantics. We do not expect the private modality representations to be fully separable in the visualization, because the instance discrimination task selected for the private space is not only related to private modality information but can also be related to the shared information across modalities. However, too much reliance on the shared information in the private space is penalized by the posed orthogonal constraints. How to design a unique proxy task that is only related to the private modality information is a challenging task that we want to investigate in the future. The margin loss solution in [1] can not be applied because we do not have downstream category information during the self-supervised pretraining.

\textcolor{blue}{Q: In line 29, the word “ignore” may not be as appropriate.}

Response: We agree with the reviewer and will change ``ignore'' to ``explicitly consider'' in our next draft.

\textcolor{blue}{Q: In the experiments, why not consider some more common multimodal scenarios, such as the MOSI [4] and MOSEI [5] datasets, which contain the three most common modalities in the real world, i.e., Language, Visual and Acoustics, and whose features are packaged as time-series-based, in line with the settings in this paper.}

Response: Thanks for the suggestion. Due to the short duration of the rebuttal period, we were not able to extend our framework to more diverse modalities (i.e., language, vision, and acoustics). We would leave this effort as one of our potential future extensions. Instead, we position FOCAL as a novel contrastive learning framework for multi-model time-series sensing signals in IoT applications and compare it with an extensive set of SOTA baselines for the same setting. 

\textcolor{blue}{Q: The public datasets lack the necessary references, please check carefully. (Line 199-206)}

Response: Thanks for pointing out the issue. Although the references are added in the Appendix, we will also add the missing references in the main body of the paper.

\textcolor{blue}{Q: Will the MOD dataset be open-released?}

Response: Yes, we do plan to release the MOD dataset upon the paper's acceptance.

\textcolor{blue}{Q: No limitations are provided in this paper.}

Response: The reviewer is friendly reminded that we have put the discussion on limitations and future extensions in Appendix G due to the space limit. We will also integrate the comments from the reviewers into more limitation discussions in the next version.

\subsection{Reviwer 8mBK}

\textcolor{blue}{Q: In the experiments, what is the intuition of the hyperparameter setting of Eq.5? Sensitivity analysis appears to be lacking.}

Response: We have added the sensitivity test and plotted the performance of FOCAL against different hyperparameters in Figure \ref{fig:sensitivity_test}, and we observe that FOCAL is generally robust against the hyperparameter selections, with less than 2\% accuracy fluctuations in all cases. For this reason, we did not perform a comprehensive hyperparameter search in our experiment.

\textcolor{blue}{Q: Whether the proposed temporal structural constraint is also applicable to other comparative learning frameworks to solve the problem of temporal information locality.}

Response: As in response to Reviewer zwVA, we applied the proposed temporal constraint to multiple contrastive learning baselines (i.e., SimCLR, MoCo, CMC, Cocoa, and GMC). Table~\ref{tab:temporal_constraints_baselines_acids} and Table~\ref{tab:temporal_constraints_baselines_pamap2} summarize the results on ACIDS and PAMAP2, and we observed up to 18.99\% improvement on ACIDS and up to 8.39\% improvement on PAMAP2 in accuracy. It validates that the temporal constraint can be used as a plugin to enhance existing contrastive learning frameworks for time-series data.

\textcolor{blue}{Q: This work is based on strong orthogonality constraints, but in fact, the performance of the FOCAL-noOrth setting has not dropped too much. I am worried whether the orthogonality assumption is too strong.}

Response: Our interpretation is the introduction of the private space brings the most performance improvement (FOCAL vs. FOCAL-noPrivate), while the orthogonality constraint further enhances the performance by pushing the two spaces to exploit unrelated semantics. As can be seen from our ablation study, FOCAL-noOrth improves significantly over FOCAL-noPrivate, while FOCAL further improves over FOCAL-noOrth, which means the orthogonality constraint contributes positively to FOCAL. Alternatively, when we replace the geometrical orthogonality with the distributional independence, FOCAL-wDistInd degrades significantly compared to FOCAL-noOrth, which means the distributional independence contributes negatively to the framework.

\textcolor{blue}{Q: Eq.4 is essentially a triplet contrastive loss, are there possible alternatives? Moreover, the value of the “margin ” does not seem to be mentioned in the paper.}

Response: We conducted a sensitivity test on the margin value in the temporal triplet loss and plotted the performance of FOCAL against different margin values in Figure \ref{fig:sensitivity_test} (d). FOCAL's accuracy changes from 95.11\% to 94.89\% on ACIDS and from 82.22\% to 84.22\% on PAMAP2, when the margin varies from 0.1 to 3. Setting the margin as 1 is overall the best strategy. We also conclude that FOCAL is not very sensitive to the temporal constraint margin selection.

\textcolor{blue}{Q: Figure 6 should be compared with the visualization results of the best baseline (or some variants of FOCAL), so as to reflect the differences or superiority. like Supervised vs. MoCo vs. FOCAL?}

Response: We provide the t-SNE visualization comparison between FOCAL and several multi-modal contrastive learning frameworks (i.e., CMC, GMC, and Cocoa). Figure \ref{fig:tsne_deepsense} and Figure \ref{fig:tsne_sw_t} visualize their concatenated modality features with DeepSense and SW-T encoder, respectively, on the MOD dataset as an example. The results show that FOCAL achieved better separation among different classes.

\begin{figure}[t!]
  \centering
  \subfigure[FOCAL]{\includegraphics[width=0.23\linewidth]{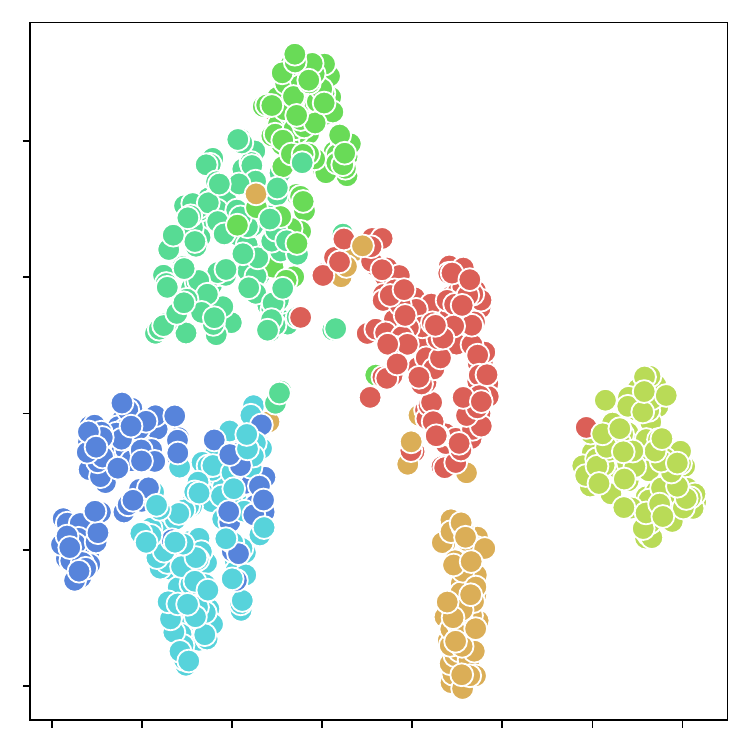}}
  \subfigure[CMC]{\includegraphics[width=0.23\linewidth]{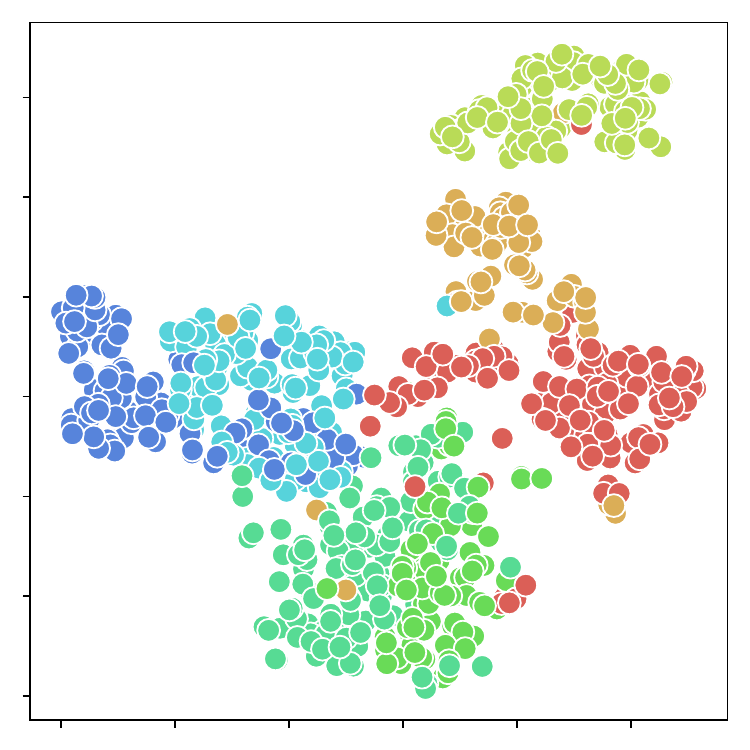}}
  \subfigure[GMC]{\includegraphics[width=0.23\linewidth]{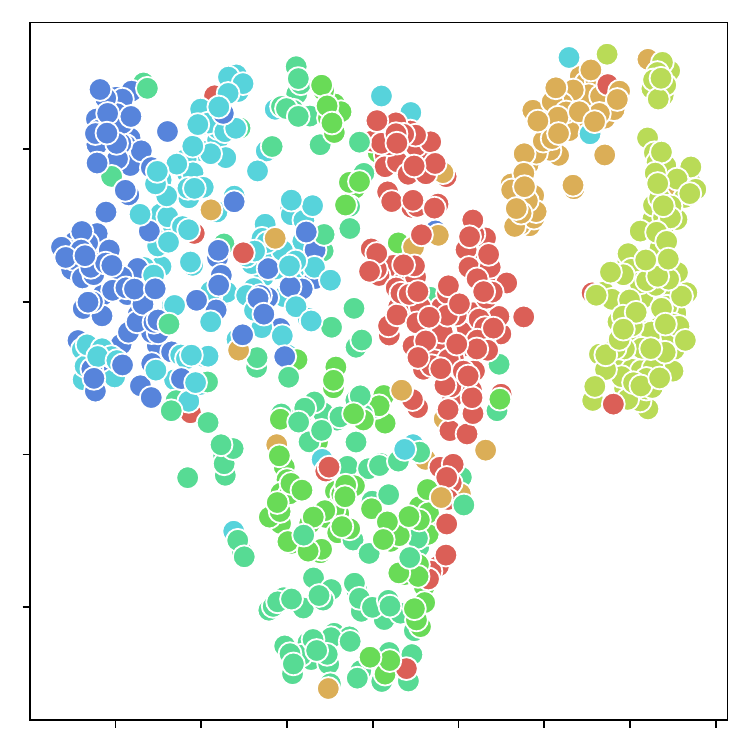}}
  \subfigure[Cocoa]{\includegraphics[width=0.23\linewidth]{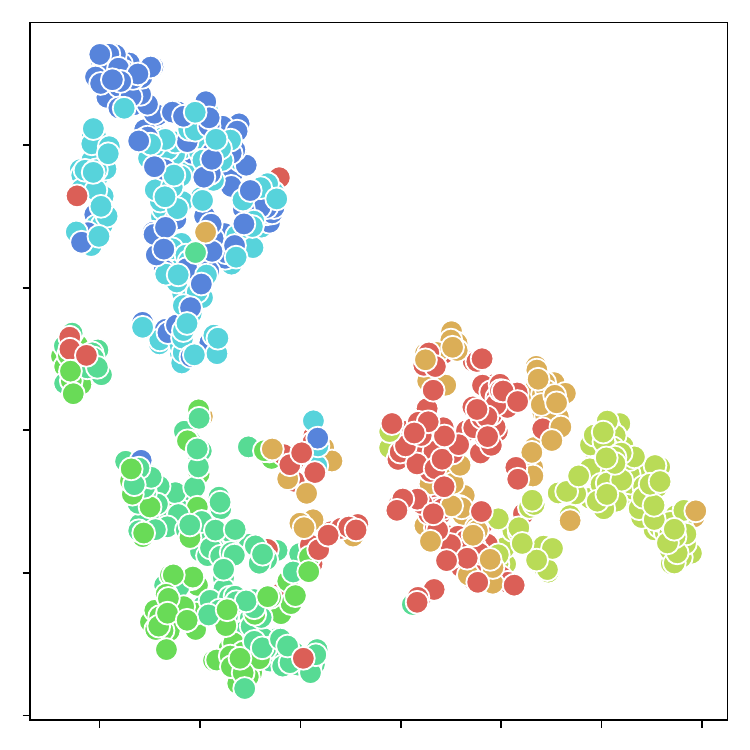}}
  \caption{t-SNE visualization of the concatenated modality features with DeepSense encoder.} 
  \label{fig:tsne_deepsense}
%  \vspace{-0.3cm}
\end{figure}

% \begin{figure}[t!]
%   \centering
  
%   \includegraphics[width=0.23\linewidth]{figure/sample_MOD_DeepSense_FOCAL.pdf}
%   % \subfigure[]{\includegraphics[width=0.23\linewidth]{figure/sample_ACIDS_DeepSense_FOCAL.pdf}}
%   % \subfigure[]{\includegraphics[width=0.23\linewidth]{figure/sample_RealWorld-HAR_DeepSense_FOCAL.pdf}}
%   % \subfigure[]{\includegraphics[width=0.23\linewidth]{figure/sample_PAMAP2_DeepSense_FOCAL.pdf}}
%   \includegraphics[width=0.23\linewidth]{figure/tsne_all/sample_MOD_DeepSense_CMC.pdf}
%   % \subfigure{\includegraphics[width=0.23\linewidth]{figure/tsne_all/sample_ACIDS_DeepSense_CMC.pdf}}
%   % \subfigure{\includegraphics[width=0.23\linewidth]{figure/tsne_all/sample_RealWorld-HAR_DeepSense_CMC.pdf}}
%   % \subfigure{\includegraphics[width=0.23\linewidth]{figure/tsne_all/sample_PAMAP2_DeepSense_CMC.pdf}}
%   \includegraphics[width=0.23\linewidth]{figure/tsne_all/sample_MOD_DeepSense_GMC.pdf}
%   % \subfigure{\includegraphics[width=0.23\linewidth]{figure/tsne_all/sample_ACIDS_DeepSense_GMC.pdf}}
%   % \subfigure{\includegraphics[width=0.23\linewidth]{figure/tsne_all/sample_RealWorld-HAR_DeepSense_GMC.pdf}}
%   % \subfigure{\includegraphics[width=0.23\linewidth]{figure/tsne_all/sample_PAMAP2_DeepSense_GMC.pdf}}
%   % \subfigure[Cosmo]{\includegraphics[width=0.23\linewidth]{figure/tsne_all/sample_MOD_DeepSense_Cosmo.pdf}}
%   % \subfigure{\includegraphics[width=0.23\linewidth]{figure/tsne_all/sample_ACIDS_DeepSense_Cosmo.pdf}}
%   % \subfigure{\includegraphics[width=0.23\linewidth]{figure/tsne_all/sample_RealWorld-HAR_DeepSense_Cosmo.pdf}}
%   % \subfigure{\includegraphics[width=0.23\linewidth]{figure/tsne_all/sample_PAMAP2_DeepSense_Cosmo.pdf}}

%   % \subfigure[MoCo]{\includegraphics[width=0.23\linewidth]{figure/tsne_all/sample_MOD_DeepSense_MoCo.pdf}}
%   % \subfigure{\includegraphics[width=0.23\linewidth]{figure/tsne_all/sample_ACIDS_DeepSense_MoCo.pdf}}
%   % \subfigure{\includegraphics[width=0.23\linewidth]{figure/tsne_all/sample_RealWorld-HAR_DeepSense_MoCo.pdf}}
%   % \subfigure{\includegraphics[width=0.23\linewidth]{figure/tsne_all/sample_PAMAP2_DeepSense_MoCo.pdf}}

%   \includegraphics[width=0.23\linewidth]{figure/tsne_all/sample_MOD_DeepSense_Cocoa.pdf}
%   % \subfigure{\includegraphics[width=0.23\linewidth]{figure/tsne_all/sample_ACIDS_DeepSense_Cocoa.pdf}}
%   % \subfigure{\includegraphics[width=0.23\linewidth]{figure/tsne_all/sample_RealWorld-HAR_DeepSense_Cocoa.pdf}}
%   % \subfigure{\includegraphics[width=0.23\linewidth]{figure/tsne_all/sample_PAMAP2_DeepSense_Cocoa.pdf}}

%   % \subfigure[Supervised]{\includegraphics[width=0.23\linewidth]{figure/tsne_all/sample_MOD_DeepSense_no.pdf}}
%   % \subfigure{\includegraphics[width=0.23\linewidth]{figure/tsne_all/sample_ACIDS_DeepSense_no.pdf}}
%   % \subfigure{\includegraphics[width=0.23\linewidth]{figure/tsne_all/sample_RealWorld-HAR_DeepSense_no.pdf}}
%   % \subfigure{\includegraphics[width=0.23\linewidth]{figure/tsne_all/sample_PAMAP2_DeepSense_no.pdf}}
% \end{figure}

\begin{figure}[t!]
  \centering
  \subfigure[FOCAL]{\includegraphics[width=0.23\linewidth]{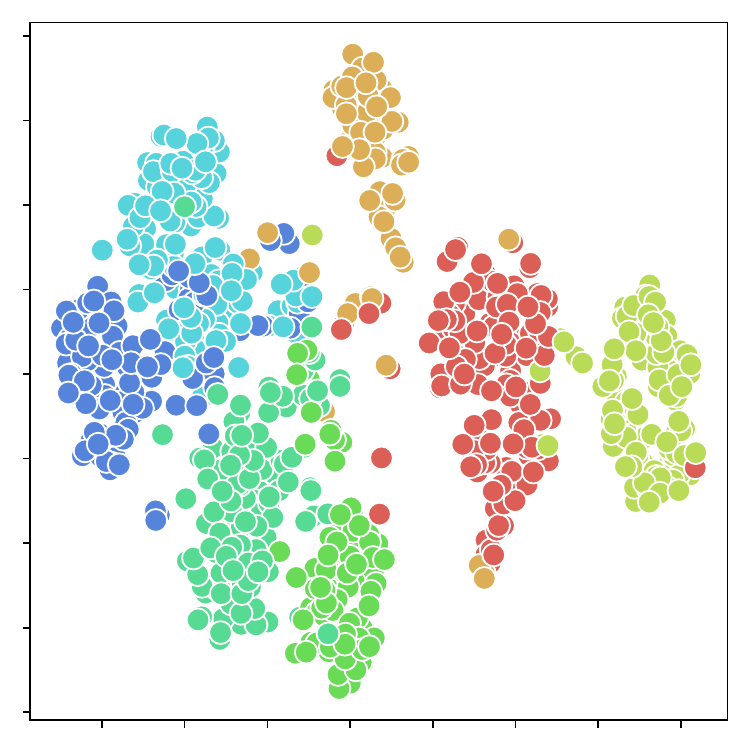}}
  \subfigure[CMC]{\includegraphics[width=0.23\linewidth]{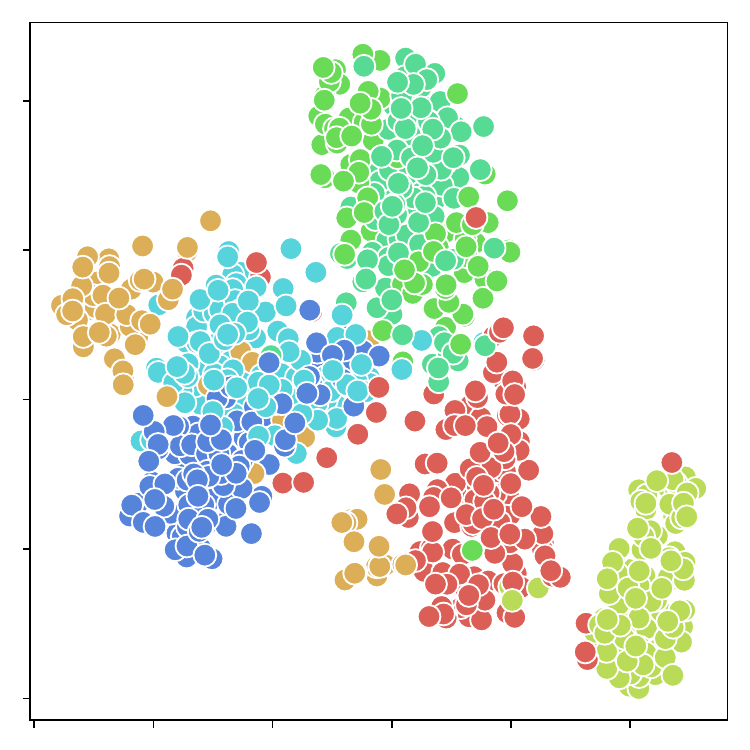}}
  \subfigure[GMC]{\includegraphics[width=0.23\linewidth]{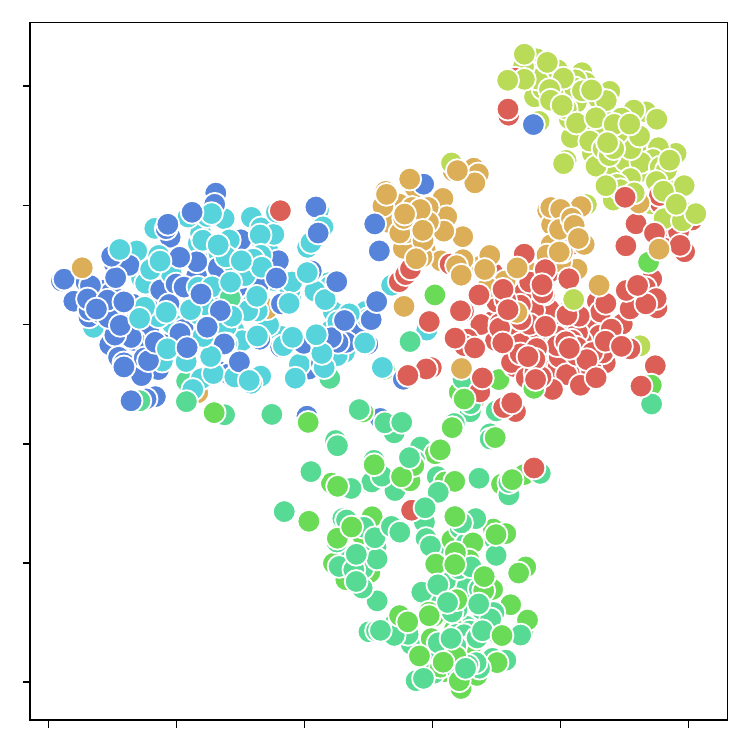}}
  \subfigure[Cocoa]{\includegraphics[width=0.23\linewidth]{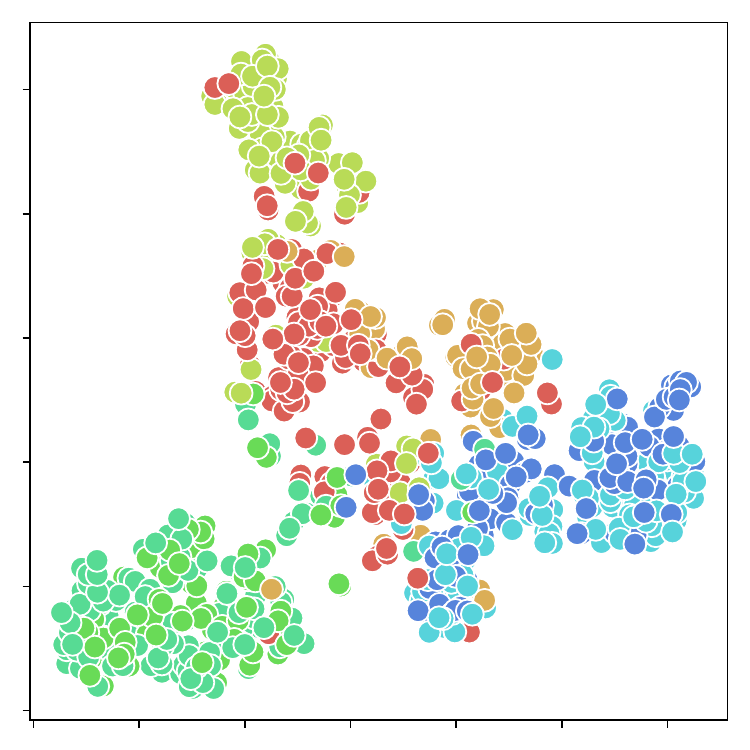}}
  \caption{t-SNE visualization of the concatenated modality features with SW-T encoder.} 
  \label{fig:tsne_sw_t}
%  \vspace{-0.3cm}
\end{figure}

% Please add the following required packages to your document preamble:
% \usepackage{booktabs}
% \usepackage{graphicx}
% Please add the following required packages to your document preamble:
% \usepackage{booktabs}
% \usepackage{graphicx}
% Please add the following required packages to your document preamble:
% \usepackage{booktabs}
% \usepackage{graphicx}
% Please add the following required packages to your document preamble:
% \usepackage{booktabs}
% \usepackage{multirow}
% \usepackage{graphicx}
% Please add the following required packages to your document preamble:
% \usepackage{booktabs}
% \usepackage{multirow}
% \usepackage{graphicx}
% Please add the following required packages to your document preamble:
% \usepackage{booktabs}
% \usepackage{multirow}
% \usepackage{graphicx}
% Please add the following required packages to your document preamble:
% \usepackage{booktabs}
% \usepackage{multirow}
% \usepackage{graphicx}
% Please add the following required packages to your document preamble:
% \usepackage{booktabs}
% \usepackage{multirow}
% \usepackage{graphicx}
\begin{table}[t!]
\centering
\caption{Benefits of Temporal Constraints to SOTA baselines on ACIDS}
\label{tab:temporal_constraints_baselines_acids}
\resizebox{\columnwidth}{!}{%
\begin{tabular}{@{}c|cc|cc|cc|cc|cc@{}}
\toprule
\multirow{2}{*}{Metrics} &
  \multicolumn{2}{c|}{SimCLR} &
  \multicolumn{2}{c|}{MoCo} &
  \multicolumn{2}{c|}{CMC} &
  \multicolumn{2}{c|}{Cocoa} &
  \multicolumn{2}{c}{GMC} \\ \cmidrule(l){2-11} 
        & Acc & F1 & Acc & F1 & Acc & F1 & Acc & F1 & Acc & F1 \\ \midrule
wTemp &
  \textbf{0.7461} &
  \textbf{0.6938} &
  \textbf{0.7836} &
  \textbf{0.6618} &
  \textbf{0.8690} &
  0.7090 &
  \textbf{0.8543} &
  \textbf{0.7665} &
  \textbf{0.9347} &
  \textbf{0.8109} \\
Vanilla & 0.7438       & 0.6101      & 0.7717       & 0.6205      & 0.8443       & \textbf{0.7244} & 0.6644       & 0.5359      & 0.9096       & 0.7929      \\ \bottomrule
\end{tabular}%
}
\end{table}

\begin{table}[t!]
\centering
\caption{Benefits of Temporal Constraints to SOTA baselines on PAMAP2}
\label{tab:temporal_constraints_baselines_pamap2}
\resizebox{\columnwidth}{!}{%
\begin{tabular}{@{}c|cc|cc|cc|cc|cc@{}}
\toprule
\multirow{2}{*}{Metrics} &
  \multicolumn{2}{c|}{SimCLR} &
  \multicolumn{2}{c|}{MoCo} &
  \multicolumn{2}{c|}{CMC} &
  \multicolumn{2}{c|}{Cocoa} &
  \multicolumn{2}{c}{GMC} \\ \cmidrule(l){2-11} 
        & Acc    & F1     & Acc    & F1     & Acc             & F1              & Acc    & F1     & Acc    & F1     \\ \midrule
wTemp &
  \textbf{0.7129} &
  \textbf{0.6884} &
  \textbf{0.7800} &
  \textbf{0.7602} &
  0.7804 &
  0.7583 &
  \textbf{0.8442} &
  \textbf{0.8146} &
  \textbf{0.8253} &
  \textbf{0.8114} \\
Vanilla & 0.6802 & 0.6583 & 0.7559 & 0.7387 & \textbf{0.7906} & \textbf{0.7706} & 0.7603 & 0.7187 & 0.8119 & 0.7860 \\ \bottomrule
\end{tabular}%
}
\end{table}

% \begin{figure}[t!]
%   \centering
%   \subfigure[FOCAL]{\includegraphics[width=0.23\linewidth]{figure/lambda_private.pdf}}
%   \subfigure[CMC]{\includegraphics[width=0.23\linewidth]{figure/lambda_private.pdf}}
%   \subfigure[GMC]{\includegraphics[width=0.23\linewidth]{figure/lambda_private.pdf}}
%   \subfigure[Cocoa]{\includegraphics[width=0.23\linewidth]{figure/lambda_private.pdf}}
%   \caption{t-SNE visualization of the concatenated modality features with SW-T encoder.} 
%   \label{fig:tsne_sw_t}
% %  \vspace{-0.3cm}
% \end{figure}

\begin{figure}[t!]
    \centering
    \includegraphics[width=1.0\linewidth]{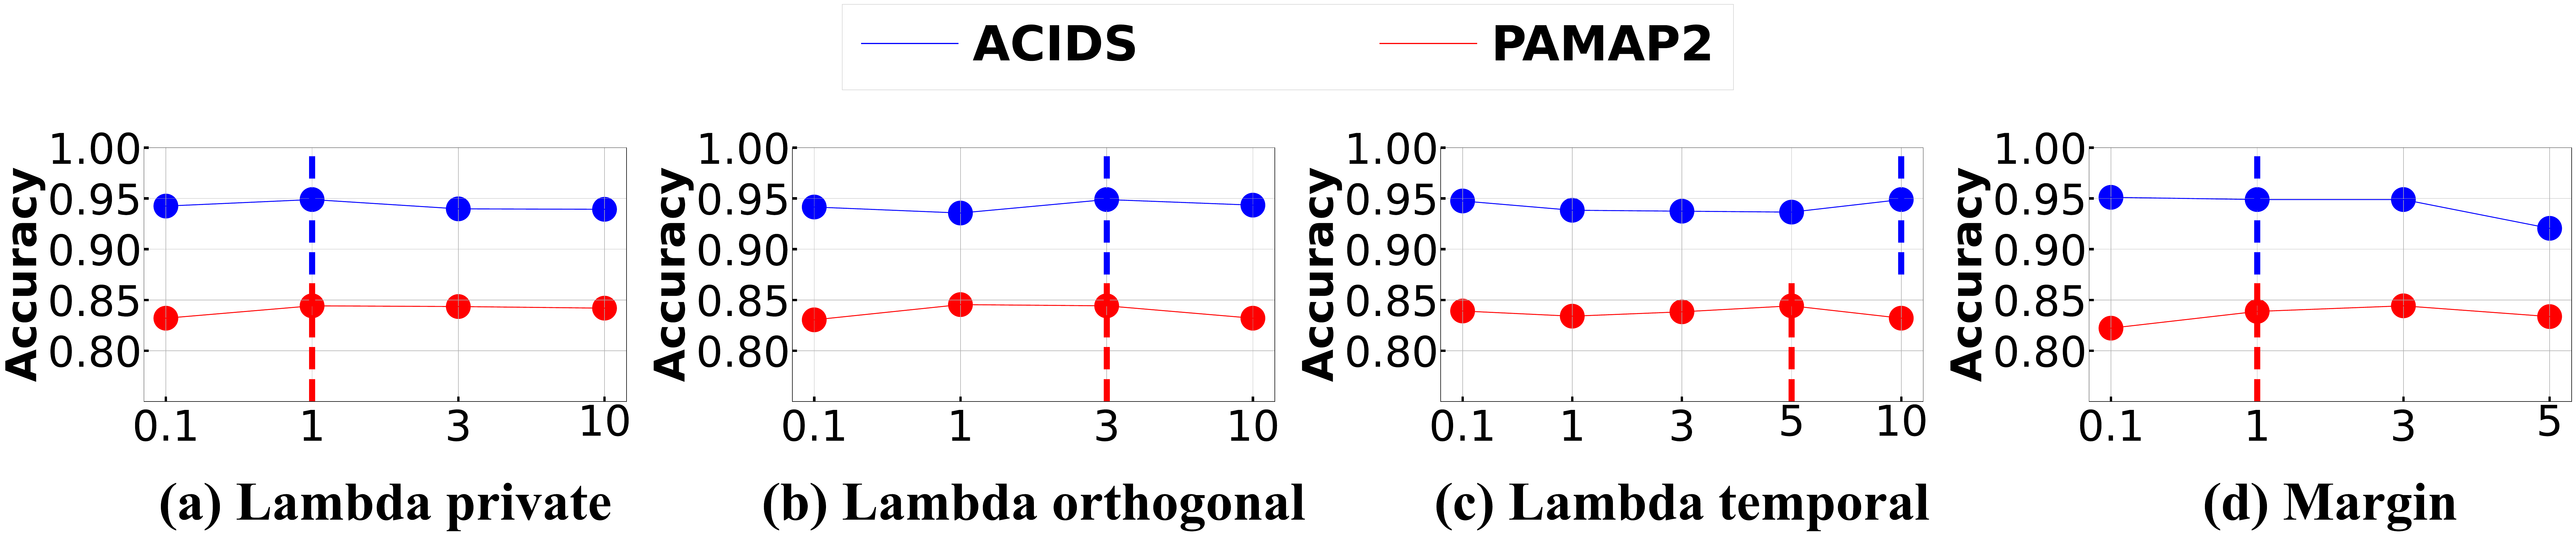}
    \caption{Loss weights sensitivity test.}
    \label{fig:sensitivity_test}
    % \vspace{4cm}
\end{figure}
% \begin{figure}[t!]
%   \centering

%   \subfigure[FOCAL]{\includegraphics[width=0.23\linewidth]{figure/sample_MOD_SW-T_FOCAL.pdf}}
%   % \subfigure[]{\includegraphics[width=0.23\linewidth]{figure/sample_ACIDS_SW-T_FOCAL.pdf}}
%   % \subfigure[]{\includegraphics[width=0.23\linewidth]{figure/sample_RealWorld-HAR_SW-T_FOCAL.pdf}}
%   % \subfigure[]{\includegraphics[width=0.23\linewidth]{figure/sample_PAMAP2_SW-T_FOCAL.pdf}}

  
%   \includegraphics[width=0.23\linewidth]{figure/tsne_all/sample_MOD_SW-T_CMC.pdf}
%   % \subfigure{\includegraphics[width=0.23\linewidth]{figure/tsne_all/sample_ACIDS_SW-T_CMC.pdf}}
%   % \subfigure{\includegraphics[width=0.23\linewidth]{figure/tsne_all/sample_RealWorld-HAR_SW-T_CMC.pdf}}
%   % \subfigure{\includegraphics[width=0.23\linewidth]{figure/tsne_all/sample_PAMAP2_SW-T_CMC.pdf}}

%   \includegraphics[width=0.23\linewidth]{figure/tsne_all/sample_MOD_SW-T_GMC.pdf}
%   % \subfigure{\includegraphics[width=0.23\linewidth]{figure/tsne_all/sample_ACIDS_SW-T_GMC.pdf}}
%   % \subfigure{\includegraphics[width=0.23\linewidth]{figure/tsne_all/sample_RealWorld-HAR_SW-T_GMC.pdf}}
%   % \subfigure{\includegraphics[width=0.23\linewidth]{figure/tsne_all/sample_PAMAP2_SW-T_GMC.pdf}}

%   % \subfigure[Cosmo]{\includegraphics[width=0.23\linewidth]{figure/tsne_all/sample_MOD_SW-T_Cosmo.pdf}}
%   % \subfigure{\includegraphics[width=0.23\linewidth]{figure/tsne_all/sample_ACIDS_SW-T_Cosmo.pdf}}
%   % \subfigure{\includegraphics[width=0.23\linewidth]{figure/tsne_all/sample_RealWorld-HAR_SW-T_Cosmo.pdf}}
%   % \subfigure{\includegraphics[width=0.23\linewidth]{figure/tsne_all/sample_PAMAP2_SW-T_Cosmo.pdf}}

%   % \subfigure[MoCo]{\includegraphics[width=0.23\linewidth]{figure/tsne_all/sample_MOD_SW-T_MoCo.pdf}}
%   % \subfigure{\includegraphics[width=0.23\linewidth]{figure/tsne_all/sample_ACIDS_SW-T_MoCo.pdf}}
%   % \subfigure{\includegraphics[width=0.23\linewidth]{figure/tsne_all/sample_RealWorld-HAR_SW-T_MoCo.pdf}}
%   % \subfigure{\includegraphics[width=0.23\linewidth]{figure/tsne_all/sample_PAMAP2_SW-T_MoCo.pdf}}

%   \includegraphics[width=0.23\linewidth]{figure/tsne_all/sample_MOD_SW-T_Cocoa.pdf}
%   % \subfigure{\includegraphics[width=0.23\linewidth]{figure/tsne_all/sample_ACIDS_SW-T_Cocoa.pdf}}
%   % \subfigure{\includegraphics[width=0.23\linewidth]{figure/tsne_all/sample_RealWorld-HAR_SW-T_Cocoa.pdf}}
%   % \subfigure{\includegraphics[width=0.23\linewidth]{figure/tsne_all/sample_PAMAP2_SW-T_Cocoa.pdf}}

%   % \subfigure[Supervised]{\includegraphics[width=0.23\linewidth]{figure/tsne_all/sample_MOD_SW-T_no.pdf}}
%   % \subfigure{\includegraphics[width=0.23\linewidth]{figure/tsne_all/sample_ACIDS_SW-T_no.pdf}}
%   % \subfigure{\includegraphics[width=0.23\linewidth]{figure/tsne_all/sample_RealWorld-HAR_SW-T_no.pdf}}
%   % \subfigure{\includegraphics[width=0.23\linewidth]{figure/tsne_all/sample_PAMAP2_SW-T_no.pdf}}
% \end{figure}
